# Supplementary material for: A Distribution Dependent and Independent Complexity Analysis of Manifold Regularization
Source: arXiv:1906.06100 ancillary file (2019-11-27)
Supplement: Supplementary file 1 [file Appendix.pdf]

# Supplementaries

## 1 Proof Theorem 2

*Proof.* First note that we can use results using  $VC$  dimension as pseudo dimension can always be formulated as the  $VC$  dimension of an appropriate set,

[Mohri et al.(2012)Mohri, Rostamizadeh, and Talwalkar, Eq. (10.4)]. First we show that an unlabeled sample size is big enough to guarantee that with probability at least  $1 - \frac{\delta}{4}$  it holds that  $\hat{R}(f_\tau^*) \leq \tau + \epsilon$ . For  $h = \text{Pdim}(\mathcal{F}, \phi)$  and  $m > h$  Theorem 5.1 from [Vapnik(1998)] states together with Sauer's Lemma that

$$P \left[ \sup_{f \in \mathcal{F}} (\hat{R}(f) - R(f)) > \epsilon \right] \leq 4e^{h-m(\epsilon-\frac{1}{m})^2}.$$

Bounding

$$4e^{h-m(\epsilon-\frac{1}{m})^2} \leq \frac{\delta}{4}$$

and rewriting this gives us that

$$m \geq \frac{1}{\epsilon^2} \left[ \ln \frac{16}{\delta} + h \ln \frac{2em}{h} + 2 \right] = \frac{1}{\epsilon^2} \left[ \ln \frac{16}{\delta} + h \ln m + h \ln \frac{2e}{h} + 2 \right]$$

is sufficient to ensure that  $\hat{R}(f) - R(f) < \epsilon$  for all  $f \in \mathcal{F}$  with probability at least  $\frac{\delta}{4}$ . Using the inequality  $\ln x \leq \alpha x - \ln \alpha - 1$  with  $x = m$  and  $\alpha = \frac{\epsilon^2}{2h}$  we can conclude that a sample of size

$$m \geq \frac{1}{\epsilon^2} \left[ \ln \frac{16}{\delta} + h \left( \frac{\epsilon^2}{2h} m + \ln \frac{2h}{\epsilon^2} - 1 \right) + h \ln \frac{2e}{h} + 2 \right] = \frac{m}{2} + \frac{1}{\epsilon^2} \left[ \ln \frac{16}{\delta} + h \ln \frac{4}{\epsilon^2} + 2 \right]$$

$\iff$

$$m \geq \frac{2}{\epsilon^2} \left[ \ln \frac{16}{\delta} + h \ln \frac{4}{\epsilon^2} + 2 \right]$$

(1)

is sufficient to guarantee  $\hat{R}(f) - R(f) < \epsilon$  for all  $f \in \mathcal{F}$  with probability at least  $\frac{\delta}{4}$ . In particular choosing  $f = f_\tau^*$  and noting that by definition  $R(f_\tau^*) \leq \tau$  we conclude that with the same probability

$$\hat{R}(f_\tau^*) \leq \tau + \epsilon. \quad (2)$$

For the second part we use the classical Hoeffding inequality with a labeled sample size of  $n$

$$P \left[ \hat{Q}(f_\tau^*) - Q(f_\tau^*) \geq \theta \right] \leq e^{-\frac{2\theta^2 n}{B^2}}.$$

Choosing  $\theta = B\sqrt{\ln(\frac{4}{\delta})\frac{1}{2n}}$  lets us conclude that with probability at least  $\frac{\delta}{4}$  it holds that

$$\hat{Q}(f_\tau^*) \leq Q(f_\tau^*) + B\sqrt{\ln(\frac{4}{\delta})\frac{1}{2n}}. \quad (3)$$

For the third part we use again Theorem 5.1 from [Vapnik(1998)], which lets us conclude that

$$P \left[ \sup_{f \in \mathcal{F}_\tau^\psi} (Q(f) - \hat{Q}(f)) > \epsilon \right] \leq 4 \text{Pdim}(\mathcal{F}, \phi) e^{-n(\frac{1}{B}(\epsilon - \frac{1}{m}))^2}.$$

Setting

$$4 \text{Pdim}(\mathcal{F}, \phi) e^{-n(\frac{1}{B}(\epsilon - \frac{1}{m}))^2} \leq \frac{\delta}{2}$$

and solving for  $n$  we conclude that a labeled sample size of

$$n \geq \frac{1}{\epsilon^2} \left[ B^2 \left( \text{Pdim}(\mathcal{F}, \phi) + \ln \frac{8}{\delta} \right) + 2 \right]$$

is sufficient to guarantee with probability at least  $\frac{\delta}{2}$  that

$$Q(f) - \hat{Q}(f) \leq \epsilon \text{ for all } f \in \mathcal{F}_{\tau+\epsilon}^\psi. \quad (4)$$

Putting everything together we get that with probability  $1 - \delta$  the classifier  $g$  that minimizes  $\hat{Q}(\cdot, X, Y)$  subject to  $\hat{R}(\cdot, U) \leq \tau + \epsilon$  satisfies

$$Q(g) \leq \hat{Q}(g) + \epsilon \leq \hat{Q}(f_\tau^*) + \epsilon \leq Q(f_\tau^*) + \epsilon + B\sqrt{\frac{\ln(\frac{4}{\delta})}{2n}}.$$

The first inequality follows from Inequality 4. The second inequality follows because  $f$  is the empirical minimizer. Note that we also need Inequality 2, i.e. that  $\hat{R}(f_\tau^*) \leq \tau + \epsilon$ , to make sure that  $f_\tau^*$  was in the search space. The third inequality follows from Inequality 3. To obtain the final inequality we use the labeled sample size to show that

$$\epsilon \geq \sqrt{\frac{1}{n} \left[ B^2 \left( \text{Pdim}(\mathcal{F}, \phi) + \ln \frac{8}{\delta} \right) + 2 \right]} \geq B \sqrt{\frac{\ln(\frac{4}{\delta})}{2n}}.$$

The first inequality holds by assumption of the labeled sample size, while the second inequality is shown by reducing it to

$$\text{Pdim}(\mathcal{F}, \phi) + 2 \geq \ln\left(\frac{\delta}{16}\right)$$

which trivially holds.

□

## References

- [Mohri et al.(2012)] Mohri, Rostamizadeh, and Talwalkar] Mehryar Mohri, Afshin Rostamizadeh, and Ameet Talwalkar. *Foundations of Machine Learning*. The MIT Press, 2012. ISBN 026201825X, 9780262018258.
- [Vapnik(1998)] Vladimir N. Vapnik. *Statistical Learning Theory*. Wiley-Interscience, 1998.
